# Supplementary material for: SEAT: Stable and Explainable Attention
Source: arXiv:2211.13290 source file (2022-11-23)
Supplement: Supplementary file 2 [file seeds_appendix.tex]

\begin{figure*}
     \centering
     \small
     \begin{tabular}{cccc}
         \includegraphics[width=3.5cm]{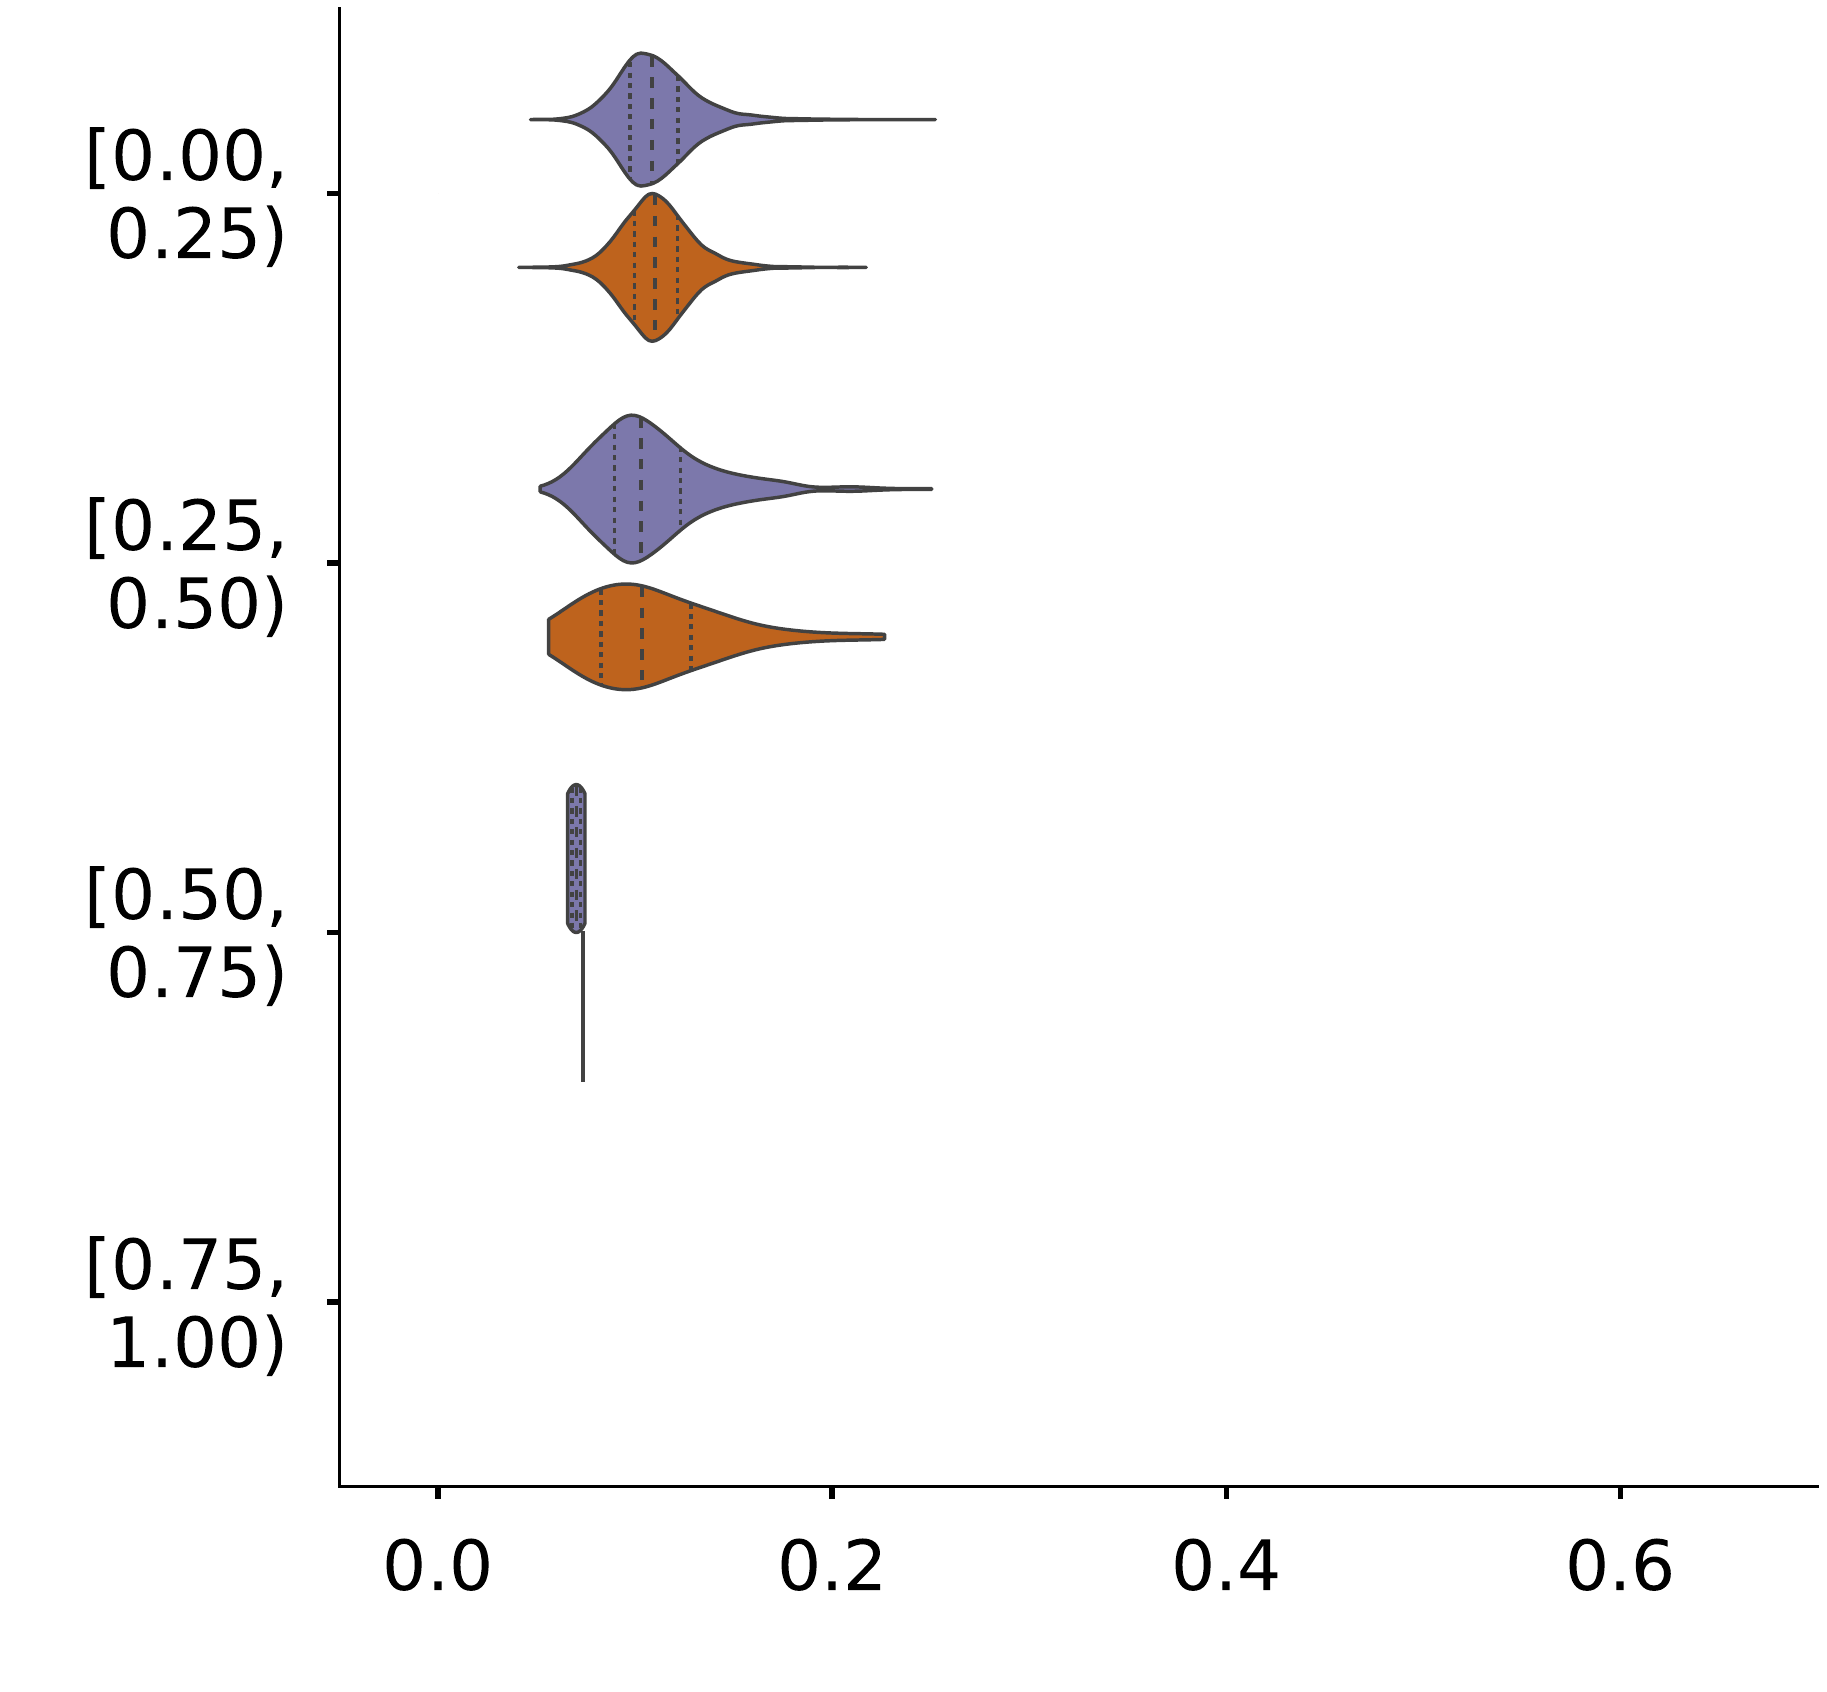}
         & 
         \includegraphics[width=3.5cm]{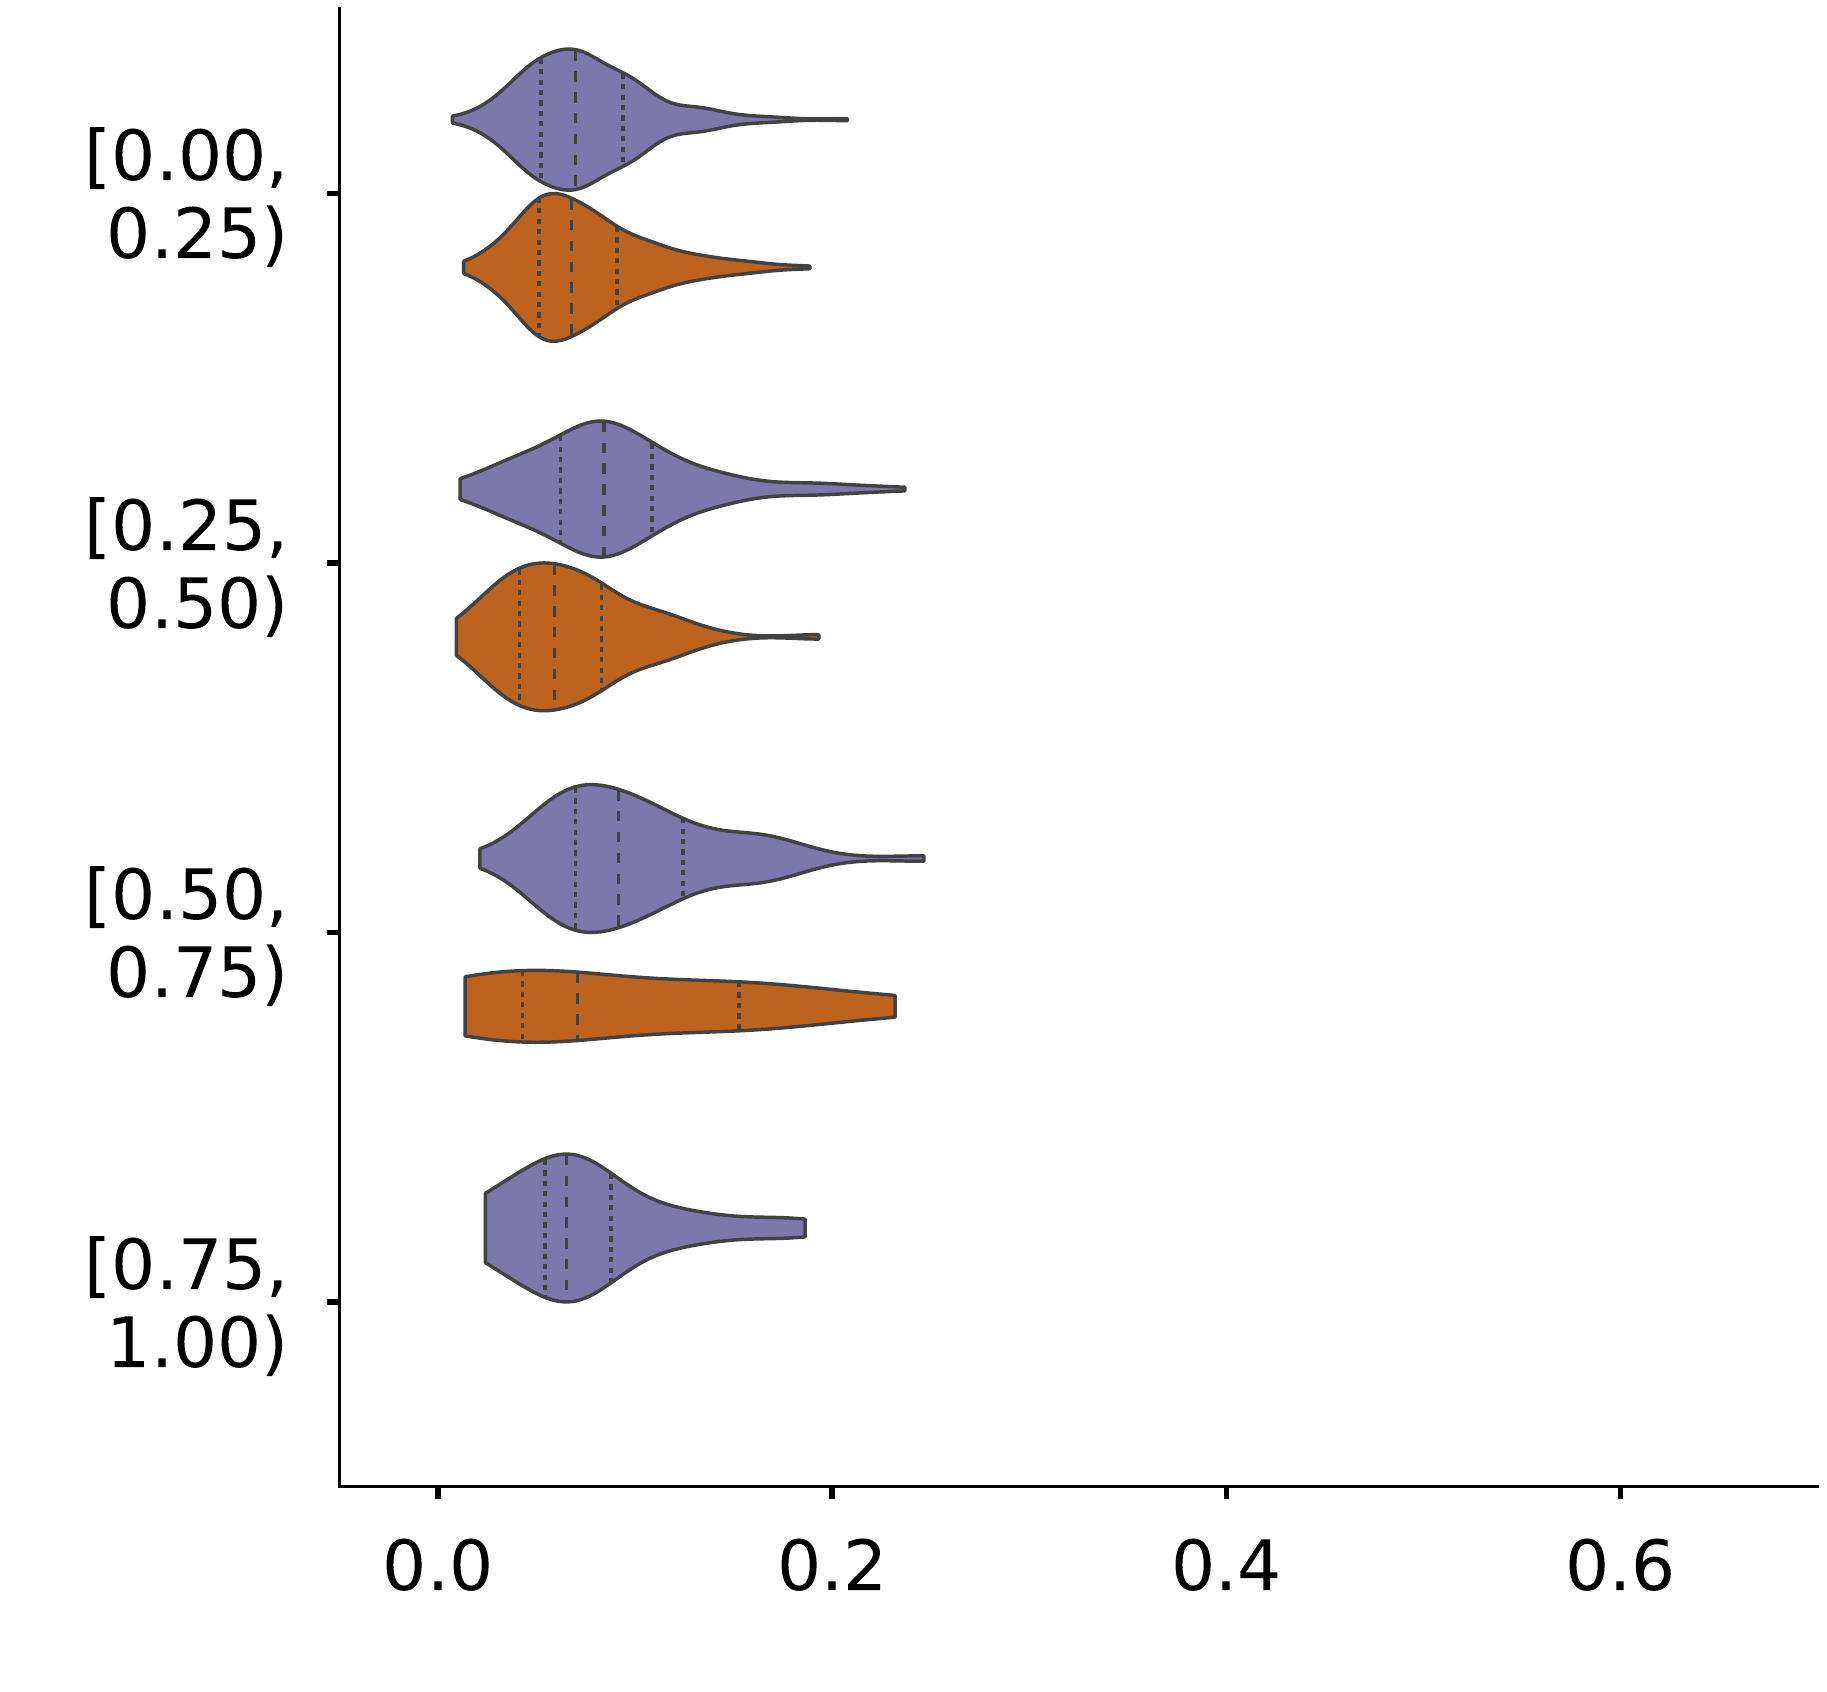}
         &
         \includegraphics[width=3.5cm]{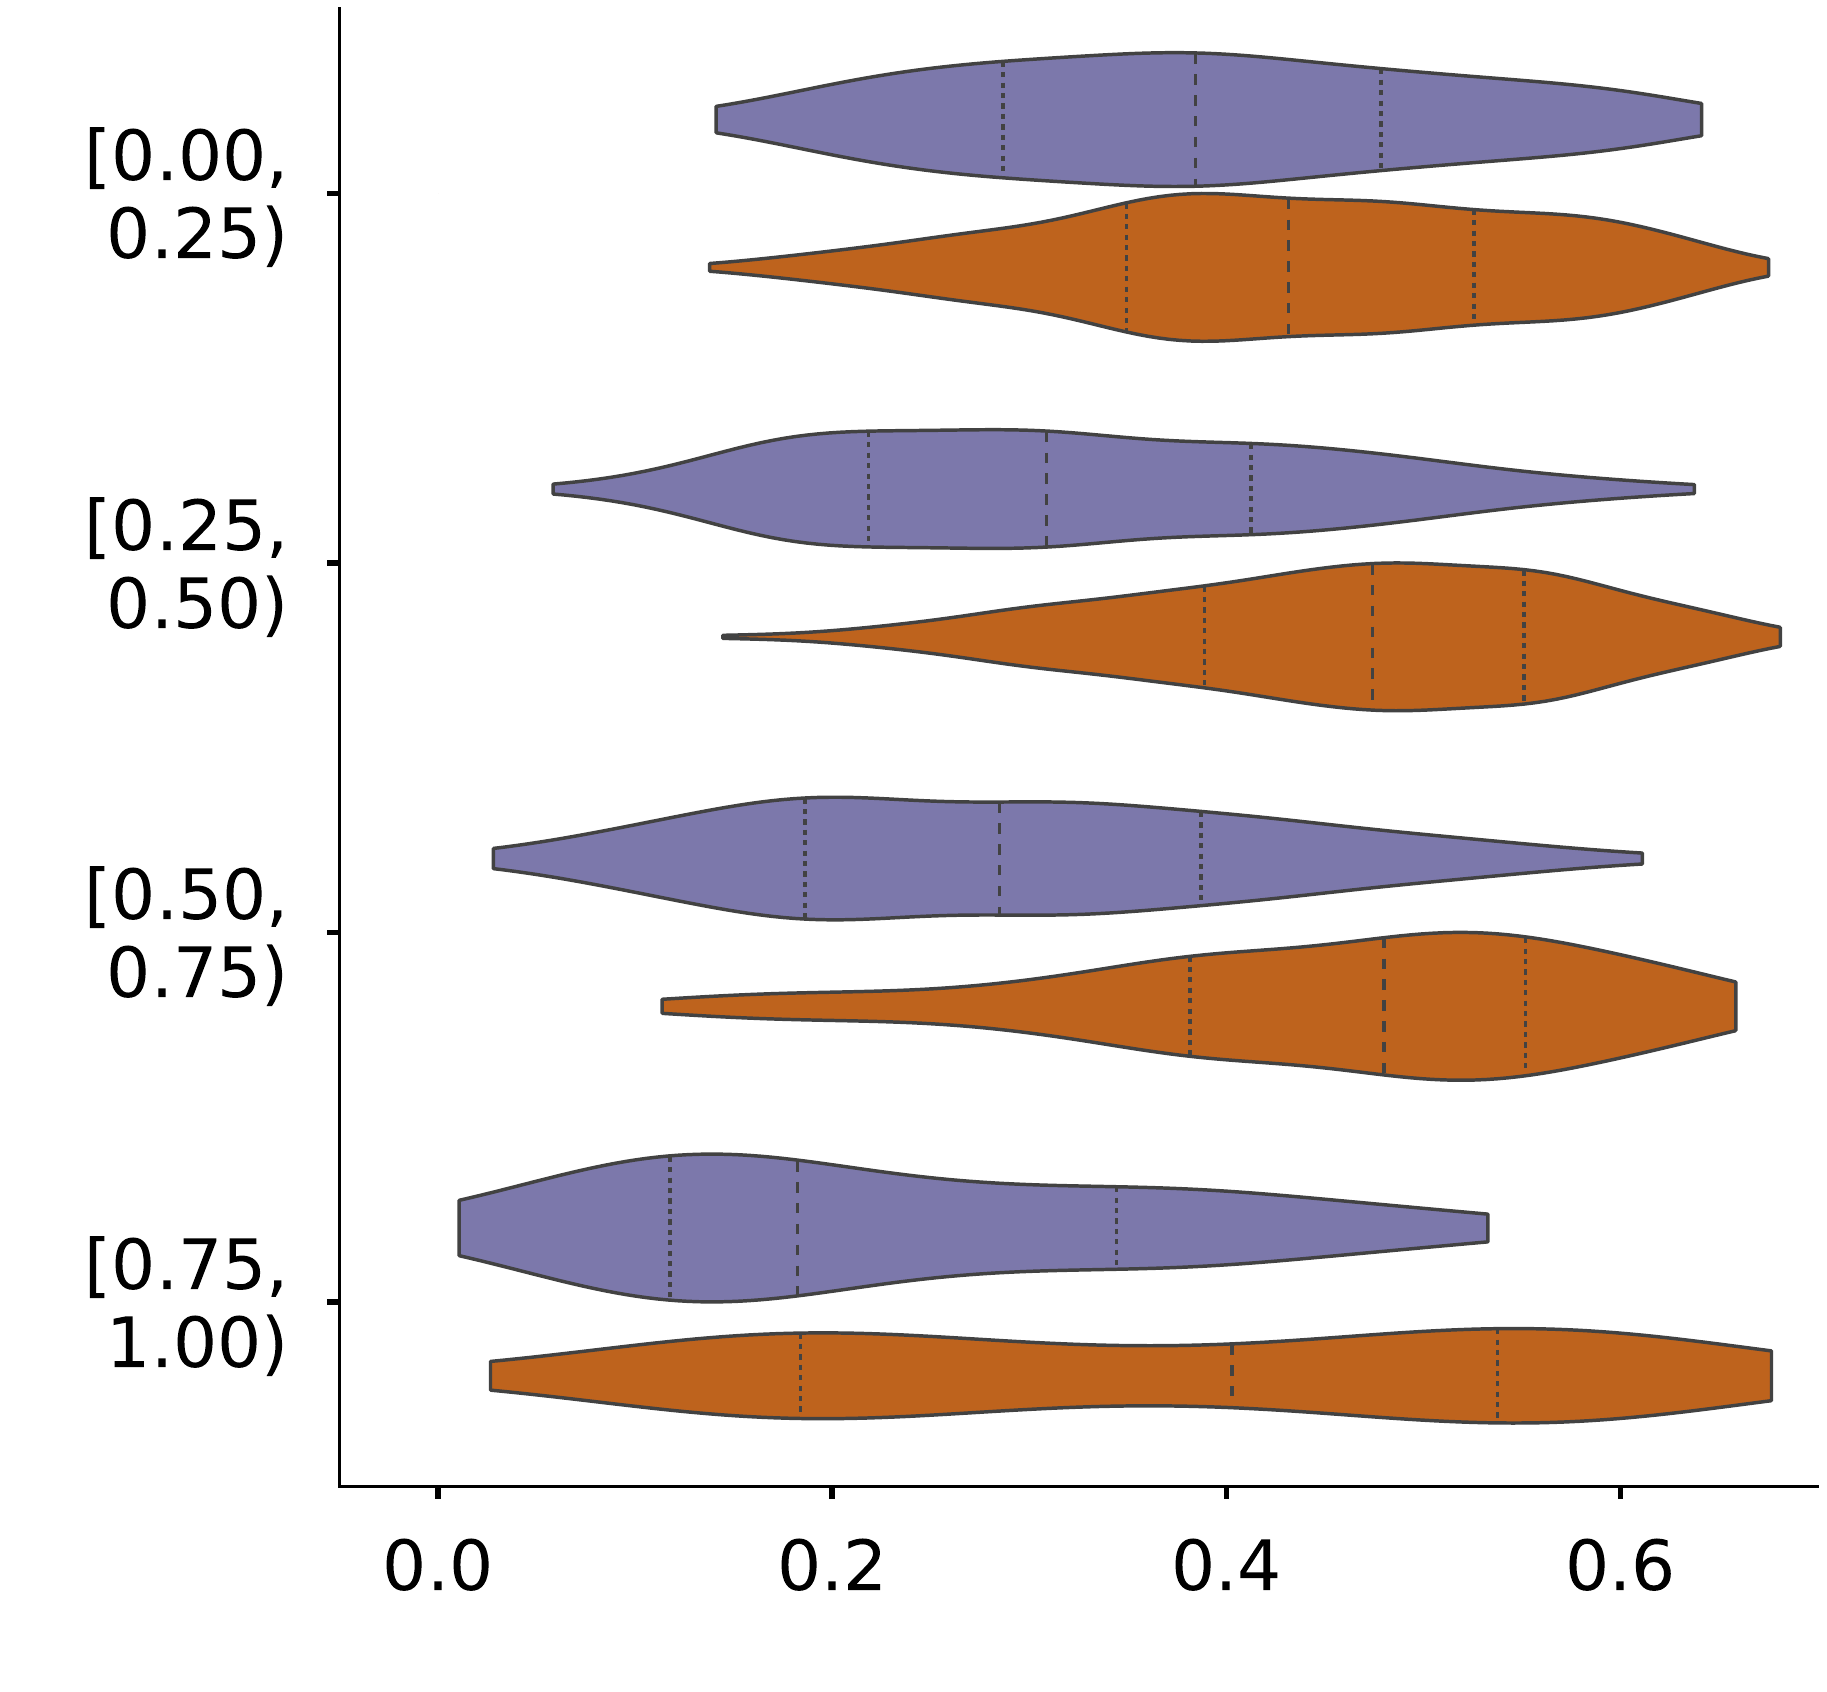}
         & 
         \includegraphics[width=3.5cm]{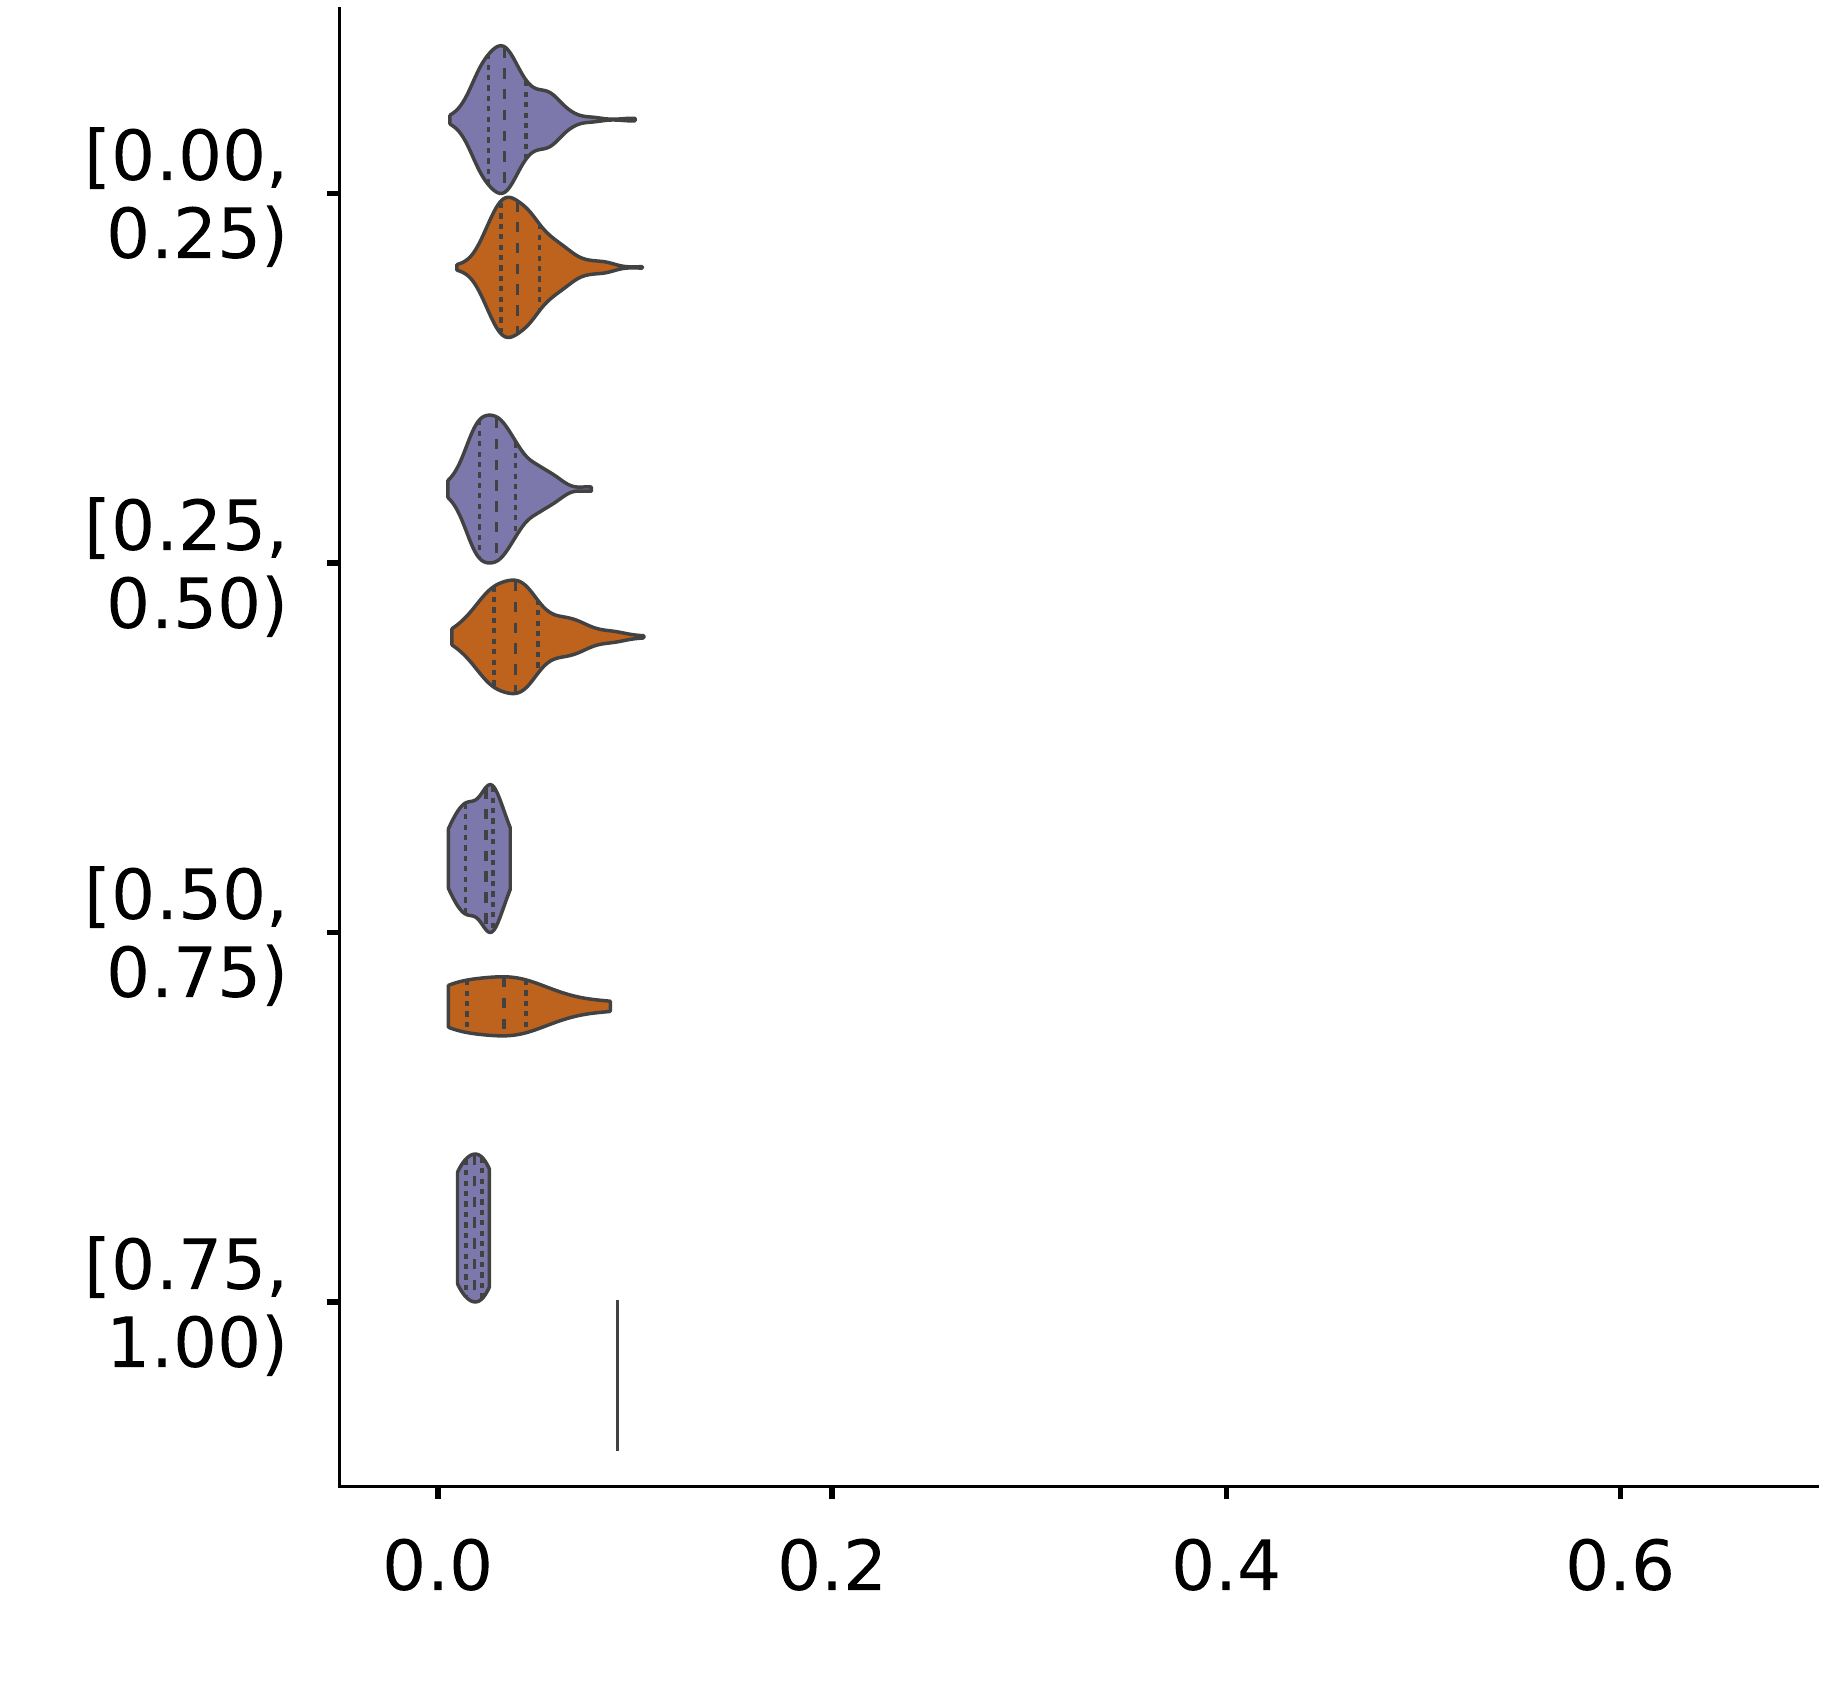} \\
         (a) Baseline-\textsc{Emotion} & (b) Baseline-SST  &
         (c) Baseline-Hate & (d) Baseline-Rotten Tomatoes \\
         \includegraphics[width=3.5cm]{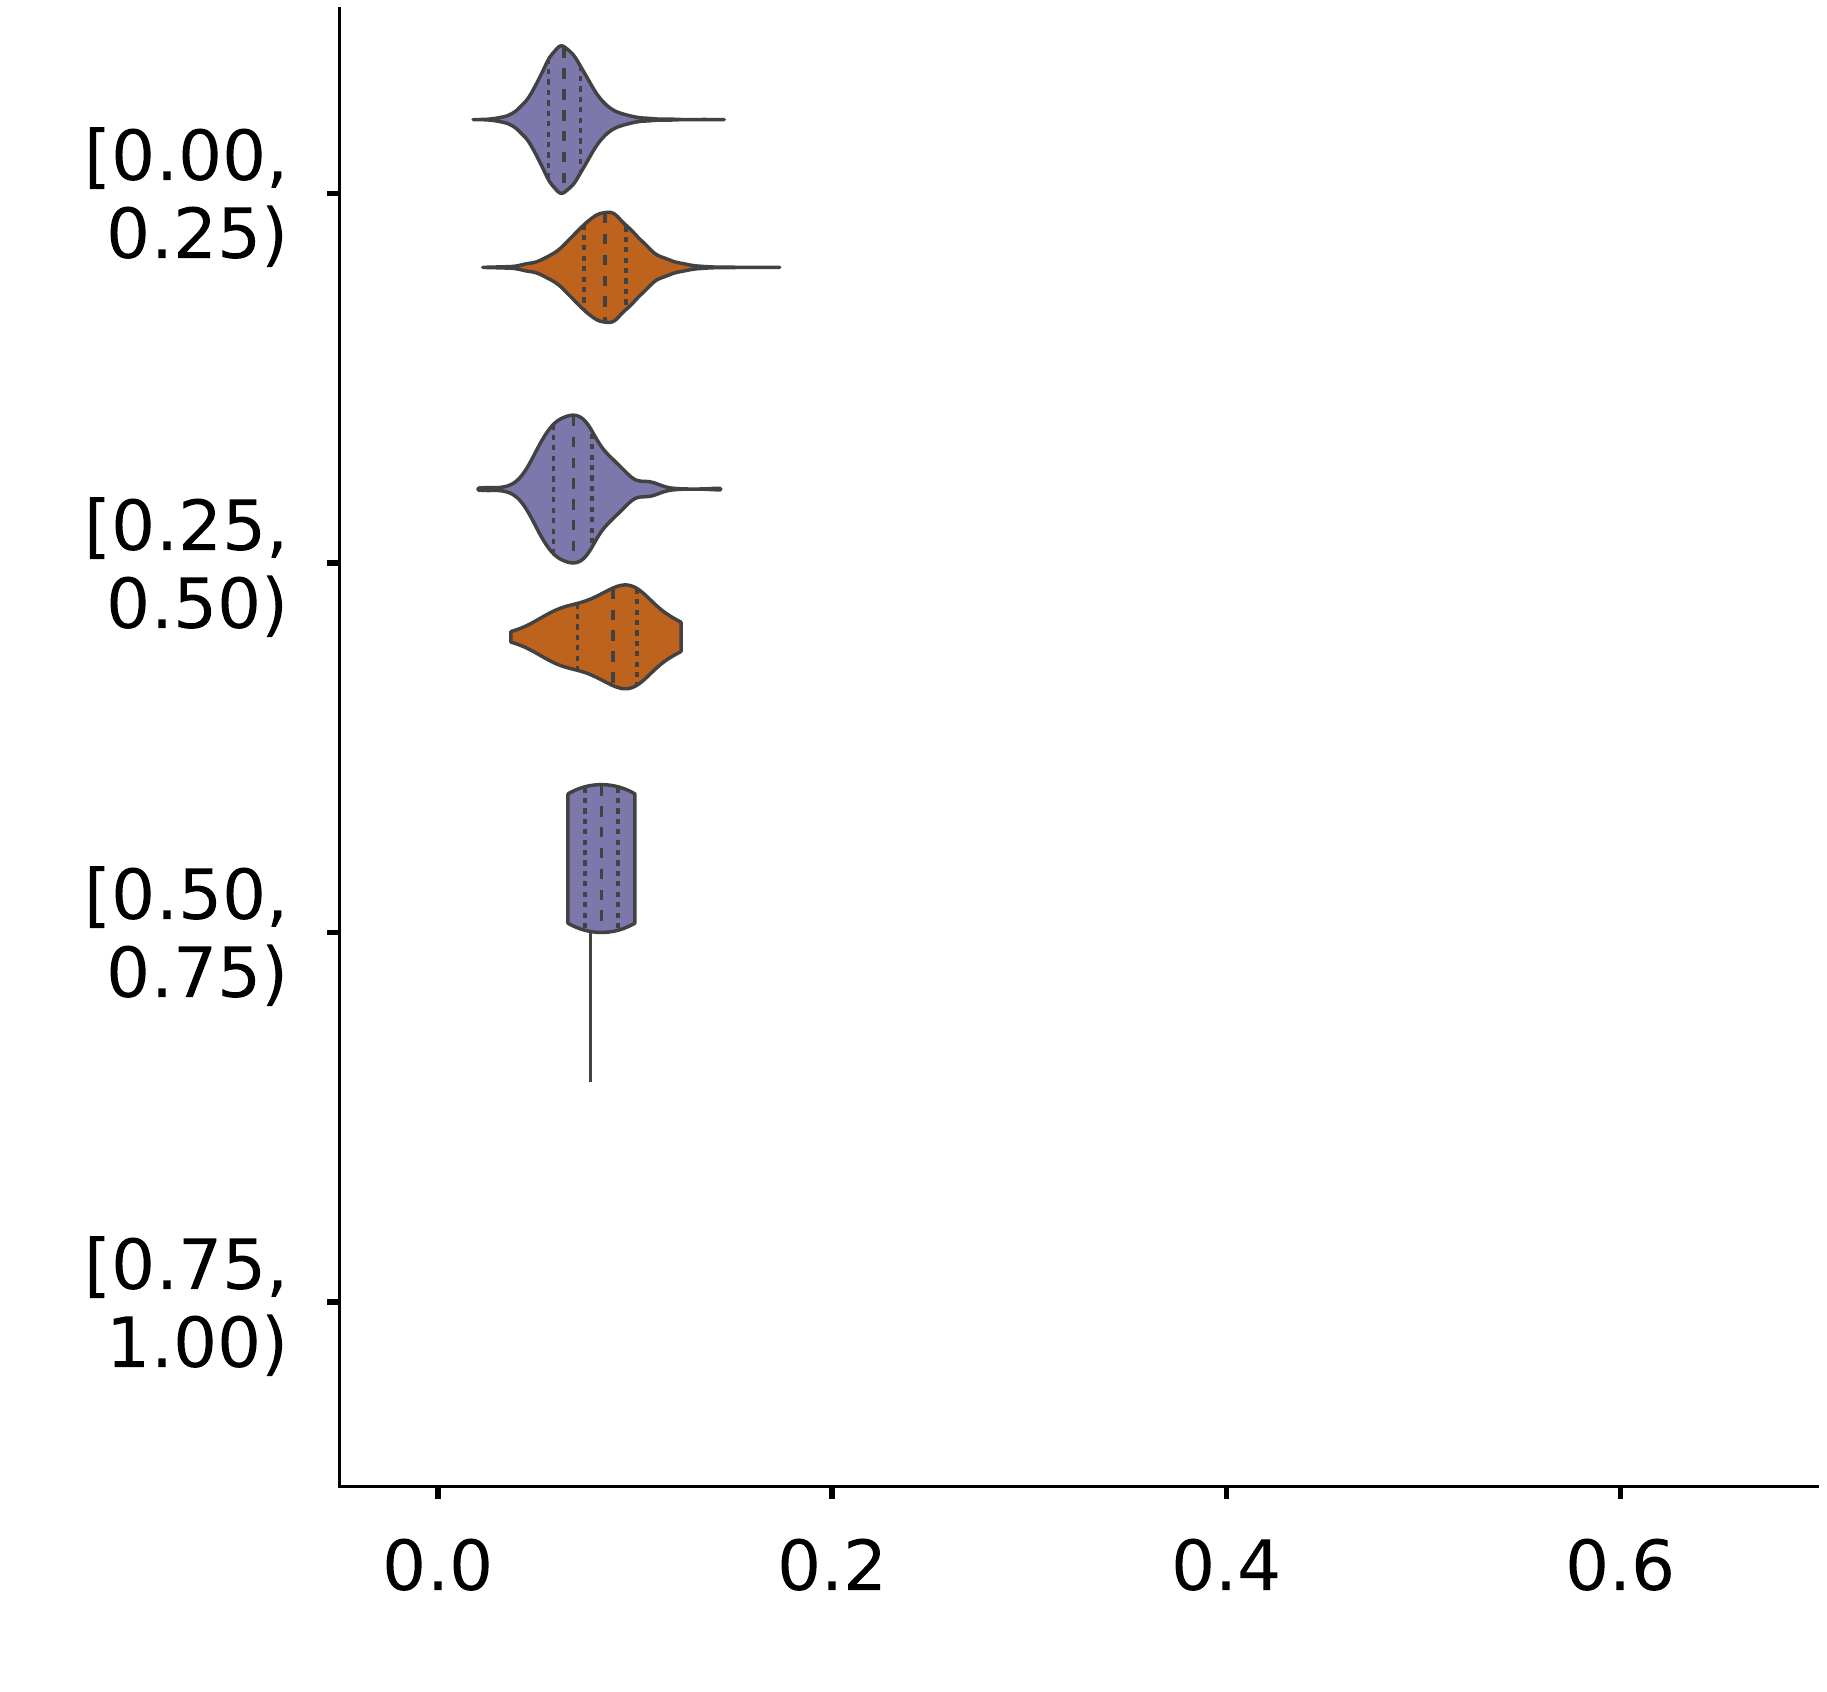}
         & 
         \includegraphics[width=3.5cm]{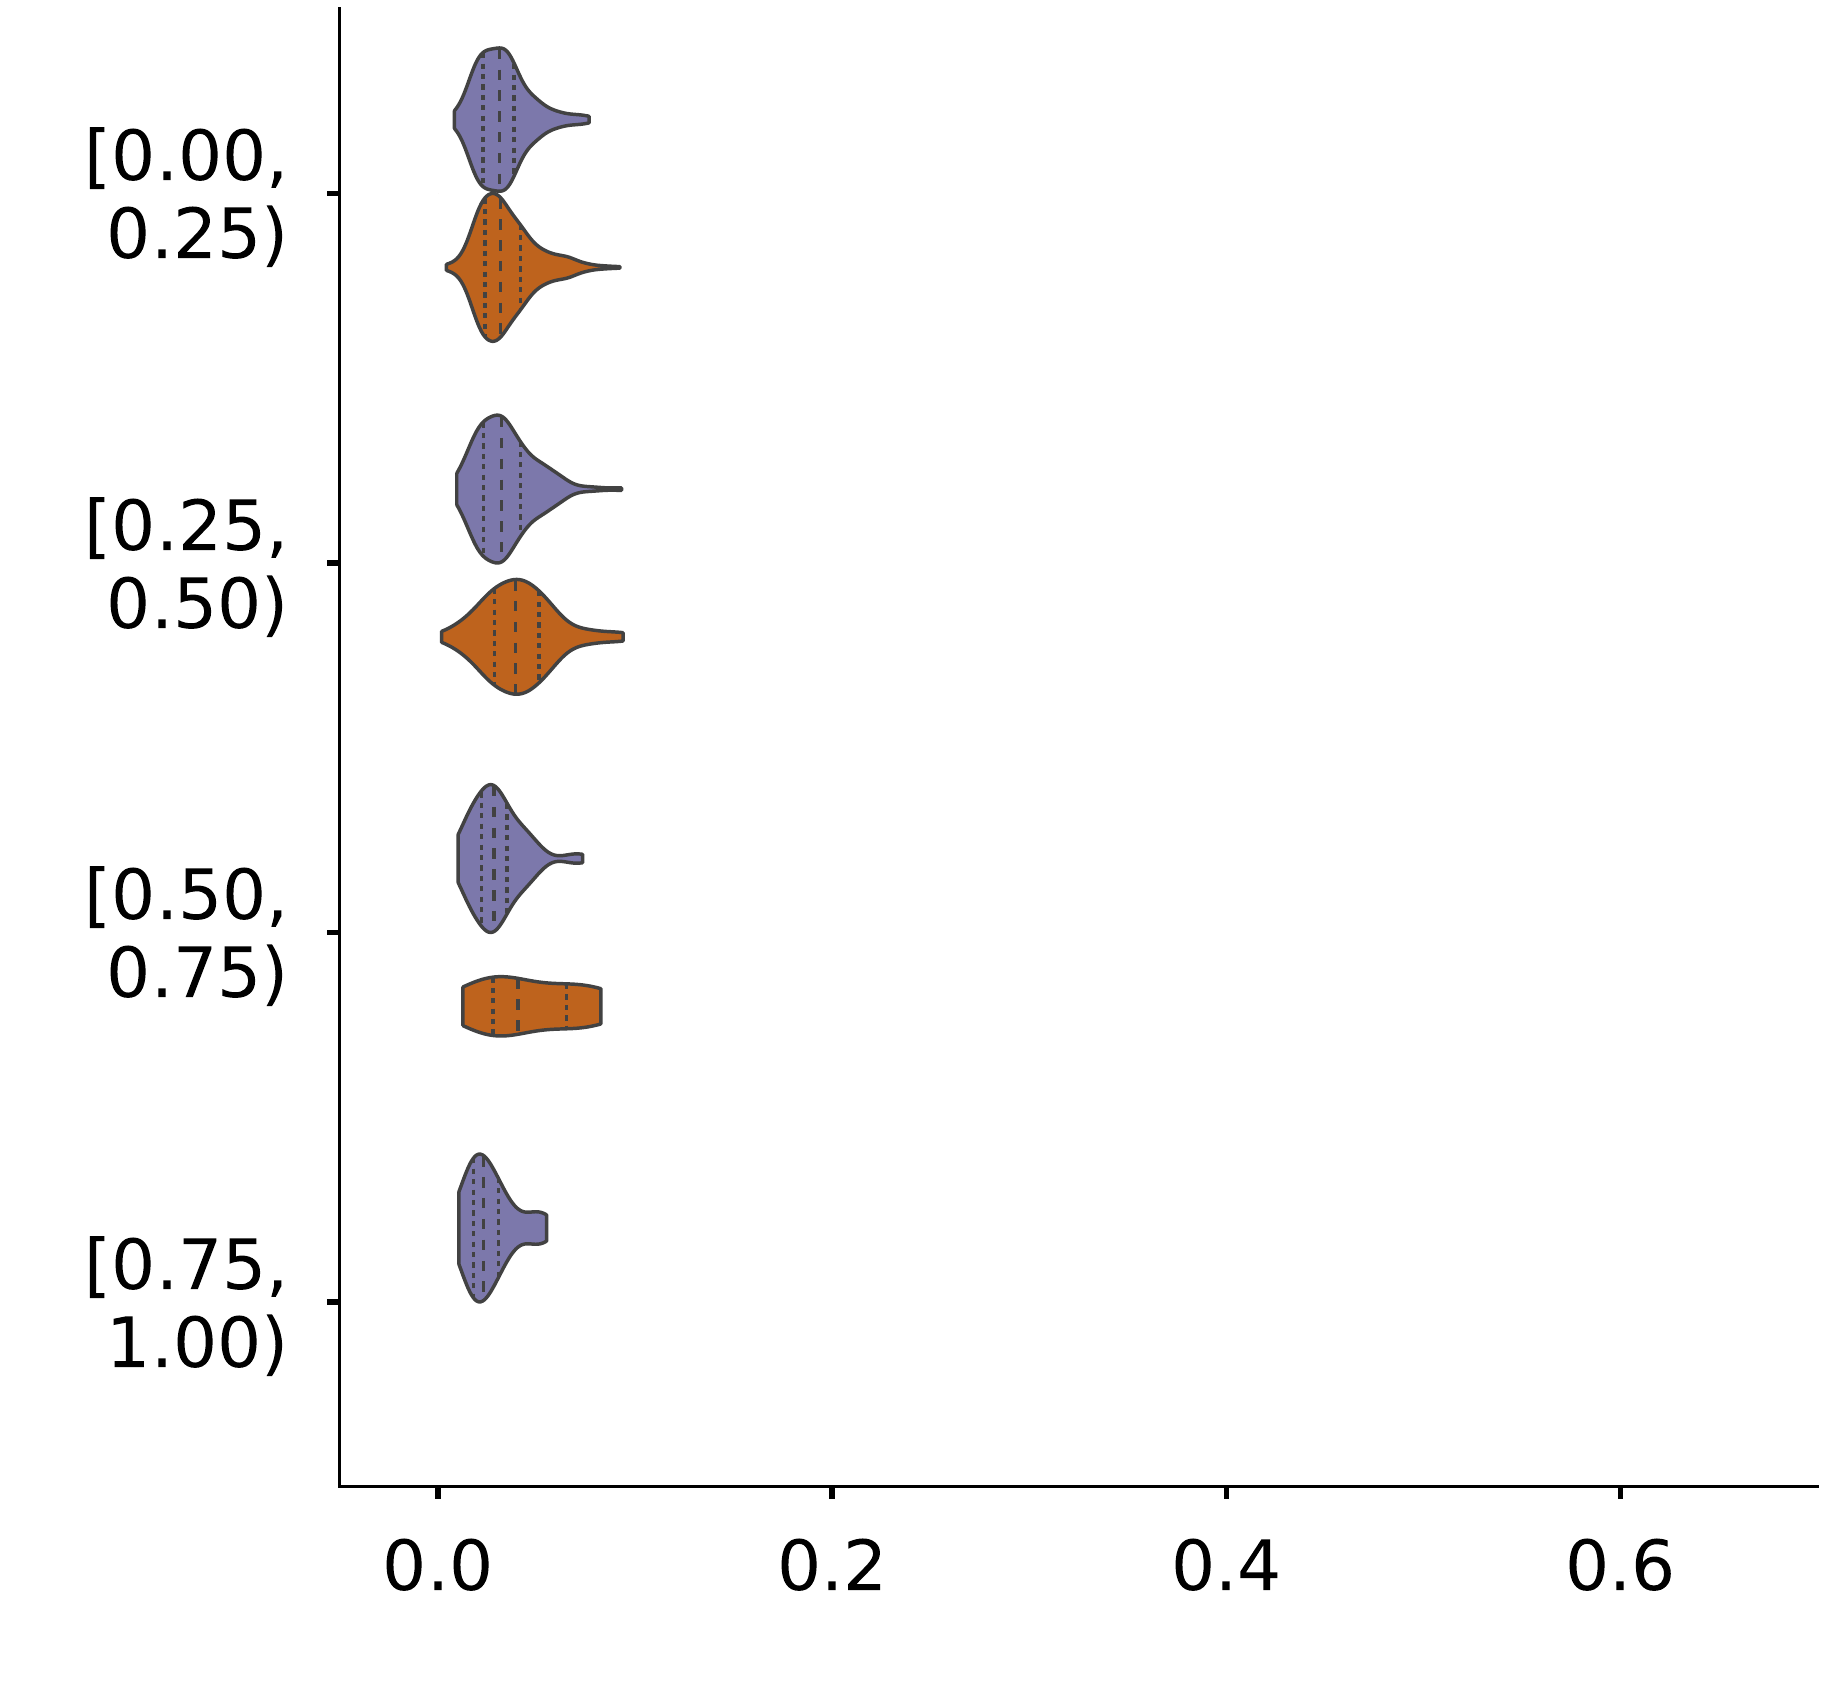} &
         \includegraphics[width=3.5cm]{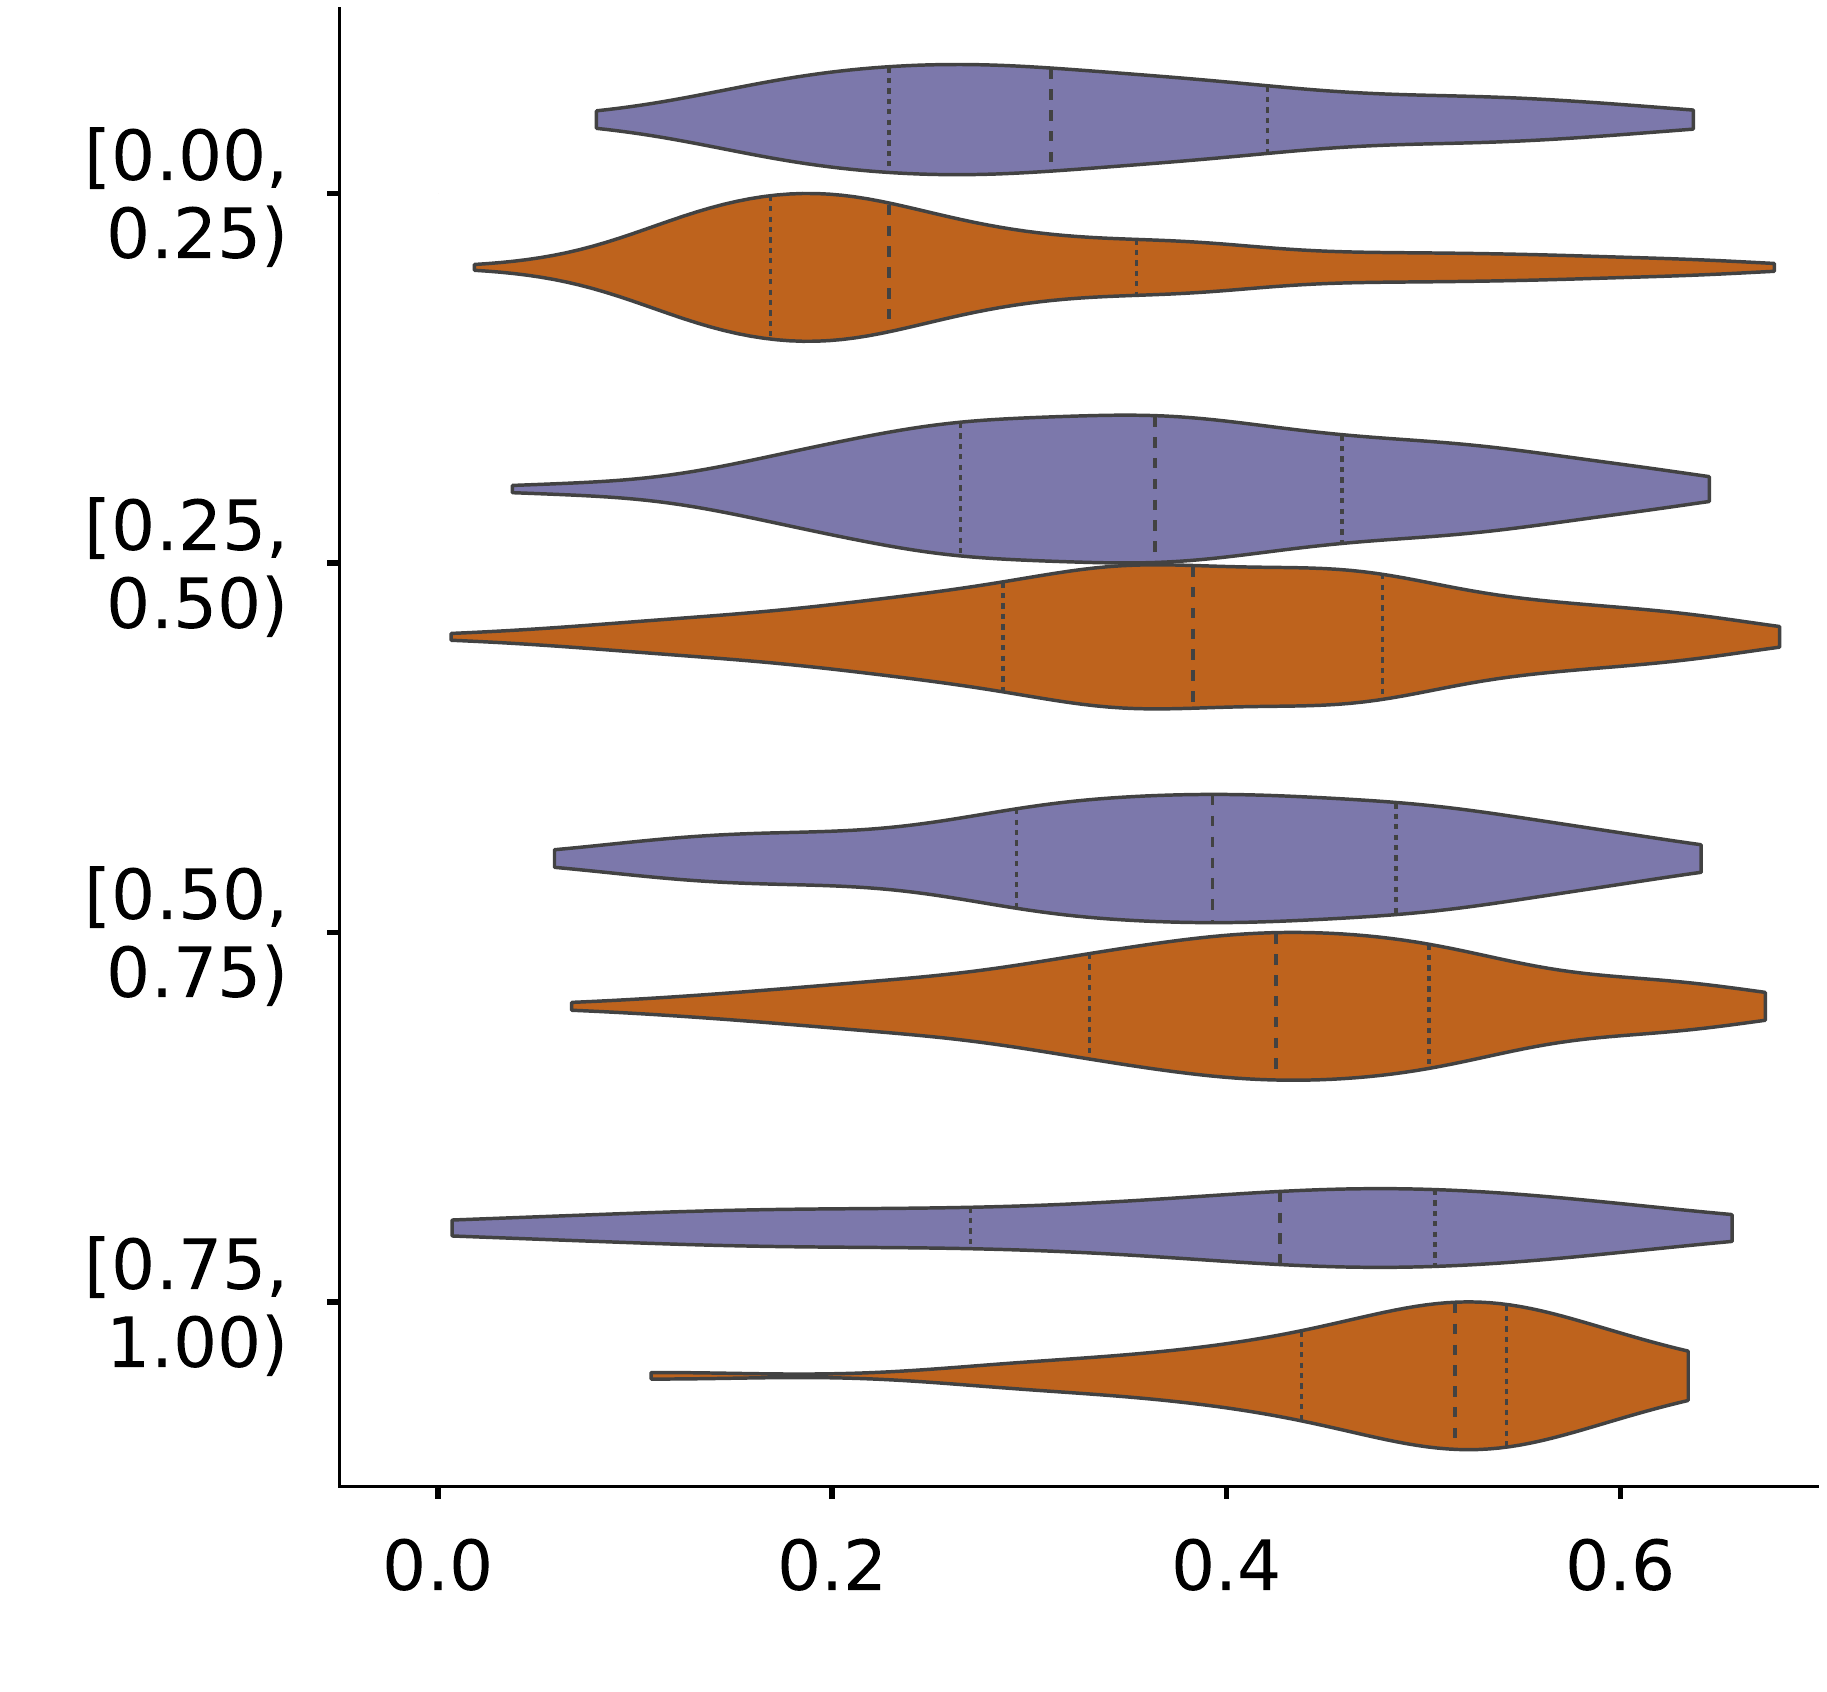}
         & 
         \includegraphics[width=3.5cm]{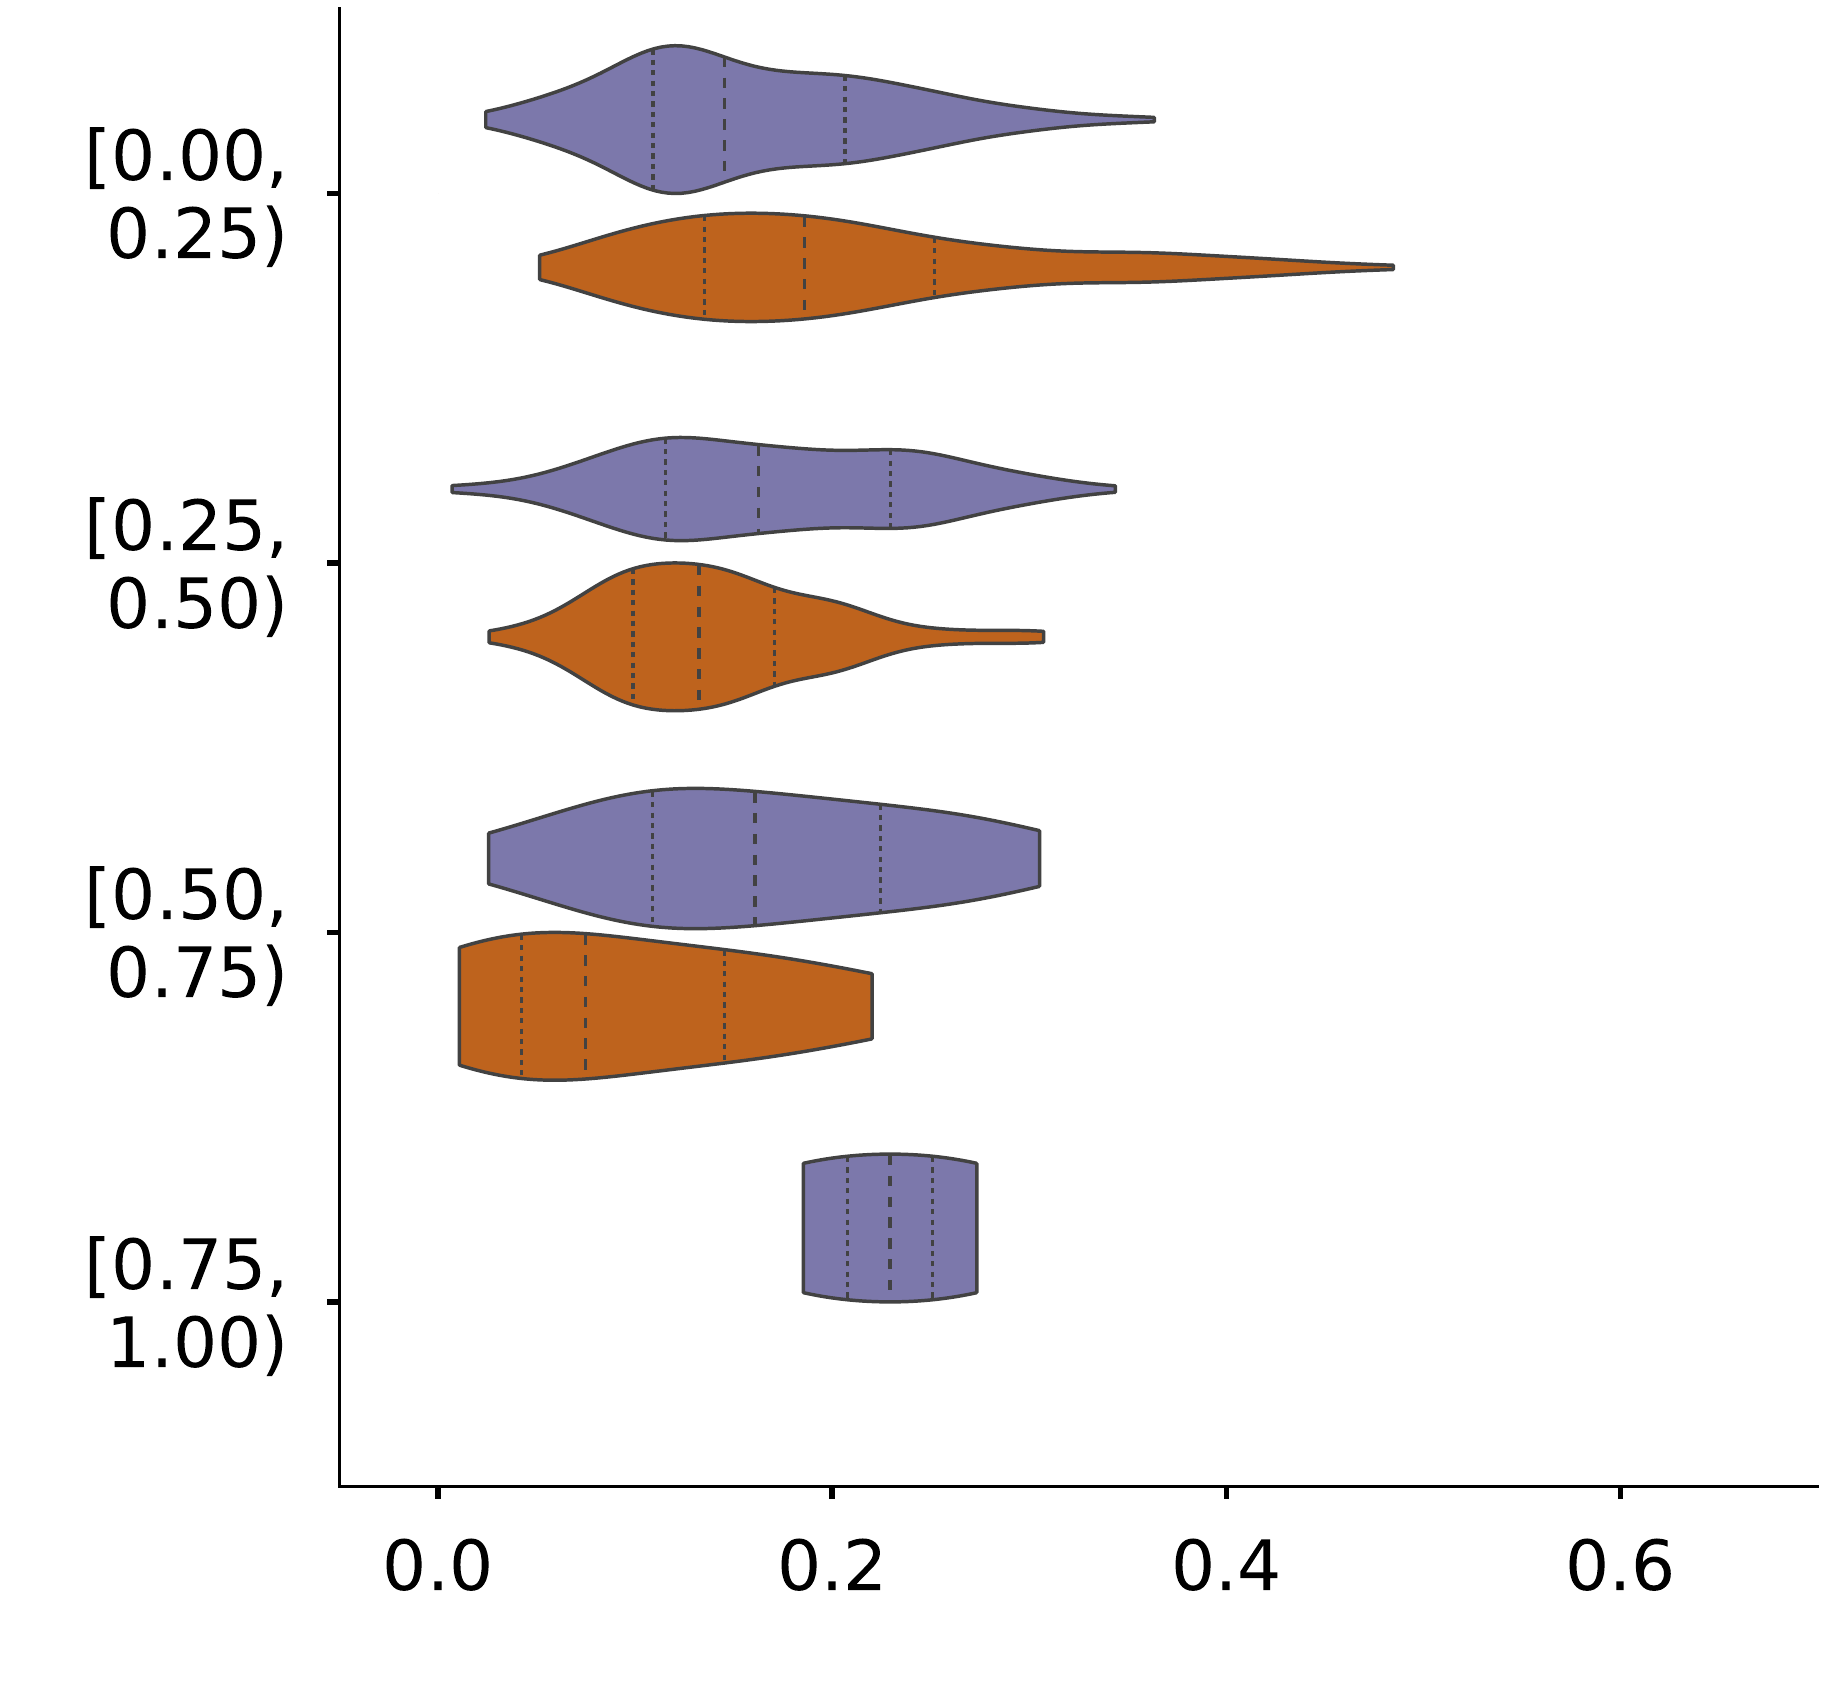} \\
         (e) Ours-\textsc{Emotion} & (f) Ours-SST  &
         (g) Ours-Hate & (h) Ours-Rotten Tomatoes \\
     \end{tabular}
     \caption{Comparison of LSTM
     Densities of maximum JS divergences (x-axis) as a function of the max attention (y-axis) in each instance between the base distributions and: (a-d) are baseline models initialized on different random seeds in four datasets; (e-h) are our attention models initialized on different random seeds in four datasets. In each max-attention bin, top (blue) is the negative-label instances, bottom (red) is positive-label instances.
     \label{fig:seeds_lstm}}
 \end{figure*}
